# Supplementary material for: The hardware is the software
Source: arXiv:2310.18335 source file (2023-10-20)
Supplement: Supplementary file 1 [file appendices.tex]

\section{Some appendix section}
\fromplm{TODO}
